# Supplementary material for: Quantum mechanics in metric space: wave functions and their densities
Source: arXiv:1102.2329 source file (2011-02-11)
Supplement: Supplementary file 1 [file supplement.pdf]

# Supplementary Information

## DEMONSTRATION THAT $D_\psi$ IS A METRIC

A metric (not to be confused with the use of the word in relativity) is a function $D(x, y)$ of two arguments that is zero only when both arguments are identical, $D(x, y) = 0 \Leftrightarrow x = y$, and satisfies the inequality, $D(x, y) \leq D(x, z) + D(y, z)$. Useful properties that follow from these two are symmetry, $D(x, y) = D(y, x)$, and positive semidefiniteness, $D(x, y) \geq 0$. This definition is therefore equivalent to using the axioms of symmetry, positive definiteness and the triangular inequality, $D(x, y) \leq D(x, z) + D(z, y)$.

A metric space is a special case of an even more fundamental concept, the topological space, in which only vicinities, but not distances, are defined.

We note that $\tilde{D}_\psi(\psi_1, \psi_2)$ may be shown to be a metric (e.g. see [1]) as it satisfies the conditions of symmetry, positive definiteness and the triangular inequality. Clearly $D_\Psi = \min_\phi \tilde{D}_\psi$ then inherits the properties of symmetry and positive definiteness of $\tilde{D}_\psi$. Then the only property which has to be proved is the triangular inequality.

For given wavefunctions we denote the phases that give the minimum distance $D_\psi$ as $\phi_A$ and $\phi_B$ and write

$$D_\psi(\Psi_1, \Psi_3) + D_\psi(\Psi_3, \Psi_2) = \min_\phi \tilde{D}_\psi(\Psi_1, \Psi_3) + \min_\phi \tilde{D}_\psi(\Psi_3, \Psi_2) \quad (1)$$

$$= \tilde{D}_\psi(\Psi_1 e^{i\phi_A}, \Psi_3) + \tilde{D}_\psi(\Psi_3, \Psi_2 e^{i\phi_B}). \quad (2)$$

As $\tilde{D}_\psi$ is a metric then it satisfies the triangular inequality so

$$\tilde{D}_\psi(\Psi_1 e^{i\phi_A}, \Psi_3) + \tilde{D}_\psi(\Psi_3, \Psi_2 e^{i\phi_B}) \geq \tilde{D}_\psi(\Psi_1 e^{i\phi_A}, \Psi_2 e^{i\phi_B}). \quad (3)$$

But we can also write the right-hand side of Eq. 3 as

$$\tilde{D}_\psi(\Psi_1 e^{i\phi_A}, \Psi_2 e^{i\phi_B}) \geq \min_\phi \tilde{D}_\psi(\Psi_1, \Psi_2), \quad (4)$$

so by considering Eqs. (1) to (4) the triangular inequality for $D_\psi$ is also satisfied and $D_\Psi$ is proven to be a metric.

## DEMONSTRATION THAT $D_\rho$ IS A METRIC

We defined the metric between any two densities as

$$D_\rho(\rho_1,\rho_2) = \int \sqrt{|\rho_1(x)|^2 + |\rho_2(x)|^2 - 2\rho_1(x)\rho_2(x)}dx = \int |\rho_1(x) - \rho_2(x)|dx. \tag{5}$$

Clearly $D_\rho$ is symmetric and positive definite. To show that it also satisfies the triangular inequality

$$D_\rho(\rho_1,\rho_2) \leq D_\rho(\rho_1,\rho_3) + D_\rho(\rho_3,\rho_2), \tag{6}$$

we can use the triangular inequality for the absolute value

$$\int |\rho_1(x) - \rho_2(x)|\, dx = \int |[\rho_1(x) - \rho_3(x)] + [\rho_3(x) - \rho_2(x)]|\, dx \tag{7}$$

$$\leq \int |\rho_1(x) - \rho_3(x)|\, dx + \int |(\rho_3(x) - \rho_2(x)|\, dx. \tag{8}$$

[1] J. von Neumann, *Mathematical Foundations of Quantum Mechanics* (reprinted by Princeton Univ. Press. 1996).
